# Supplementary material for: Attentive Knowledge-aware Graph Convolutional Networks with Collaborative Guidance for Personalized Recommendation
Source: arXiv:2109.02046 source file (2022-01-02)
Supplement: Supplementary file 1 [file appendix.tex]

\appendix
\setcounter{table}{0} 
\setcounter{figure}{0}

\section{Supplemental Results of CG-KGR Evaluation}
\label{app:results}
\subsection{CG-KGR Model Performance with Different Aggregators}

\subsubsection{\textbf{Top-$K$ Recomendation Results of Different Aggregators.}}

Detailed Top-$K$ recomendation results of Recall and NDCG \textit{w.r.t} aggregator \textit{sum}, \textit{concat}, and \textit{neigh} are shown in Figure~\ref{fig:topk_aggregator}.   
\begin{figure*}[hb]
\hspace{-0.15in}
  \subfigure[ \quad Music]{  
    \begin{minipage}{0.235\textwidth}
      \includegraphics[width=1.75in]{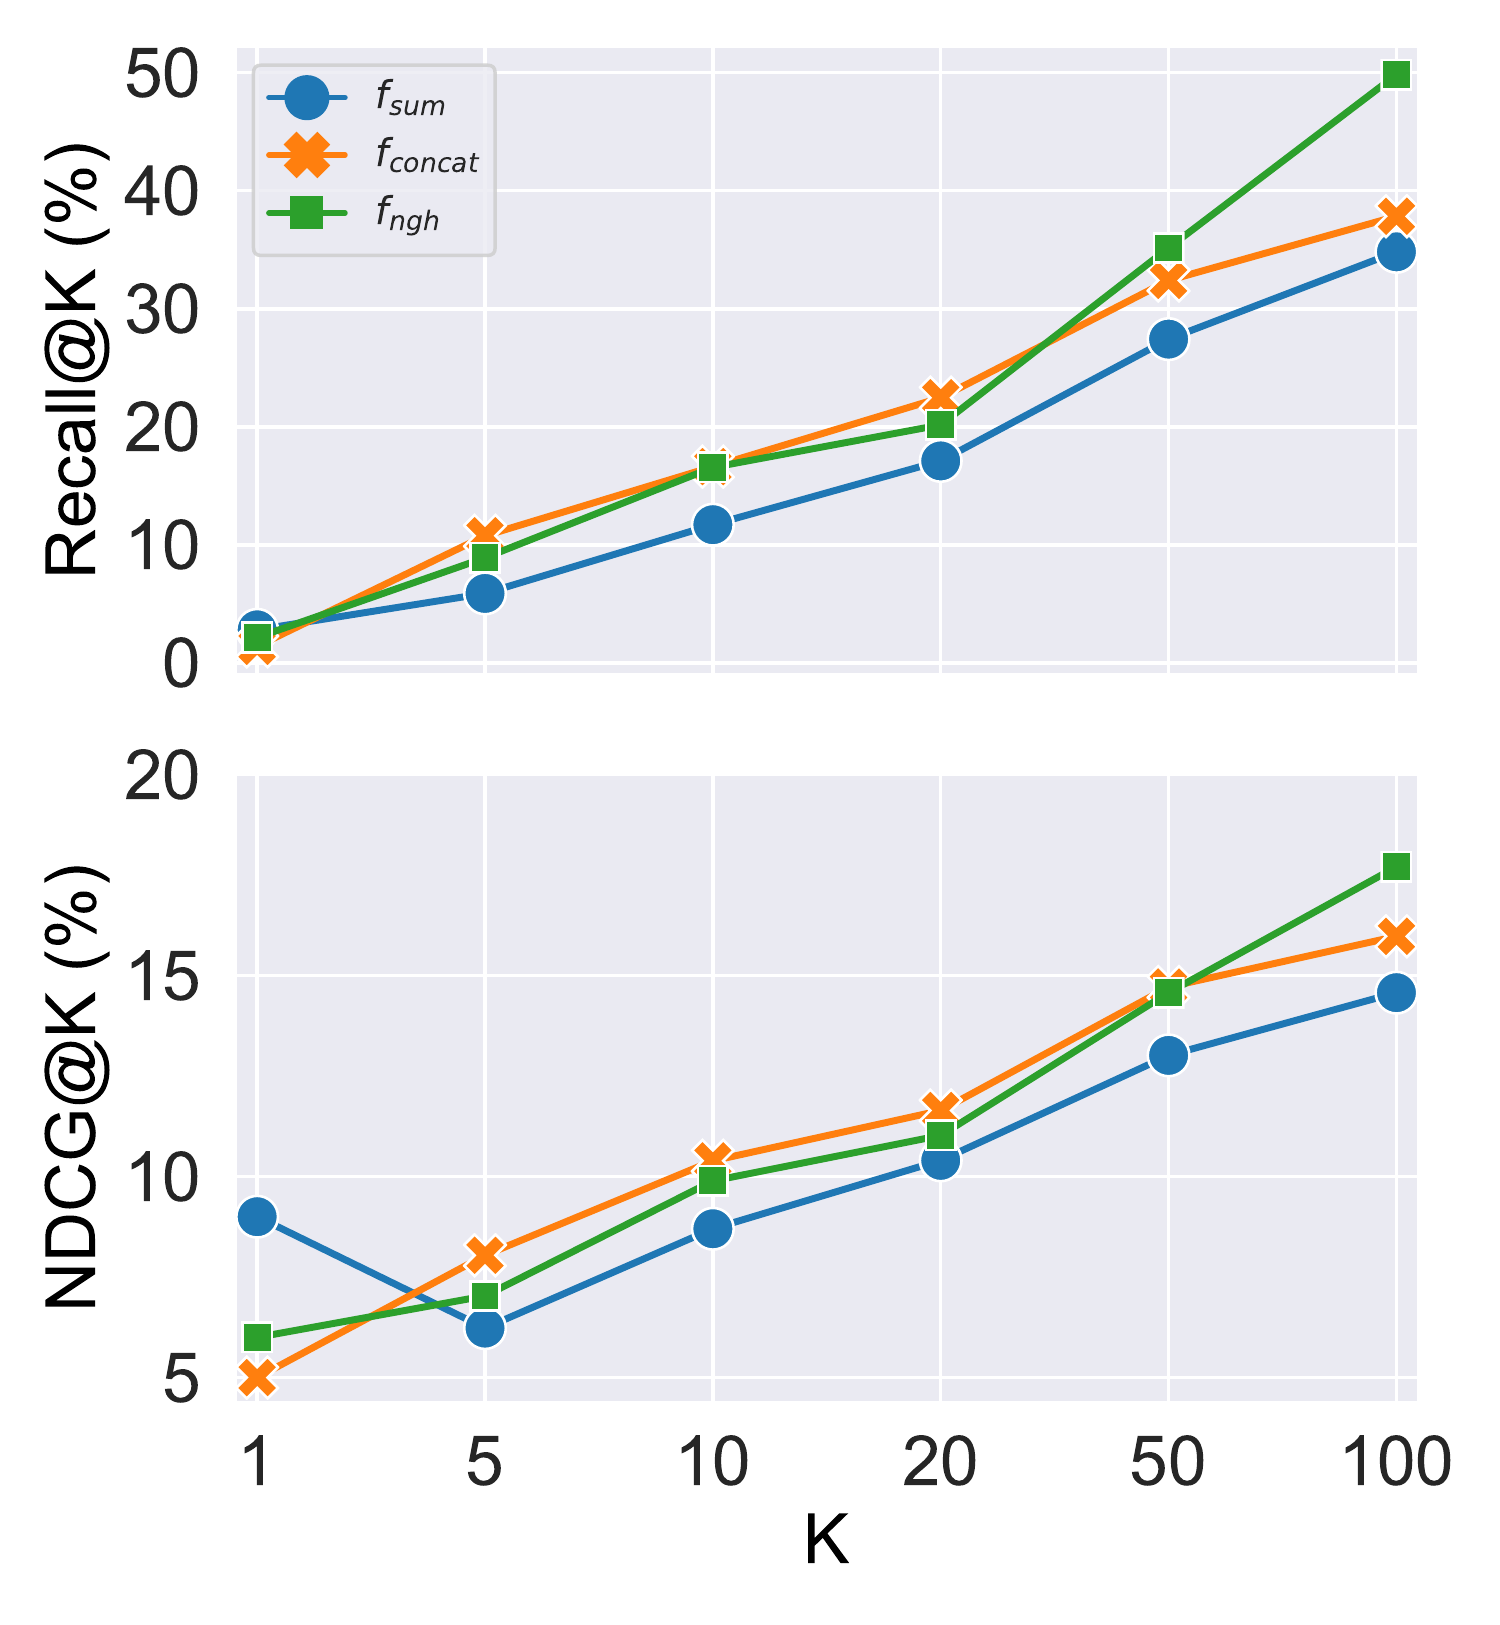}
    \end{minipage}
    }
  \subfigure[ \quad Book]{  
    \begin{minipage}{0.235\textwidth}
      \includegraphics[width=1.75in]{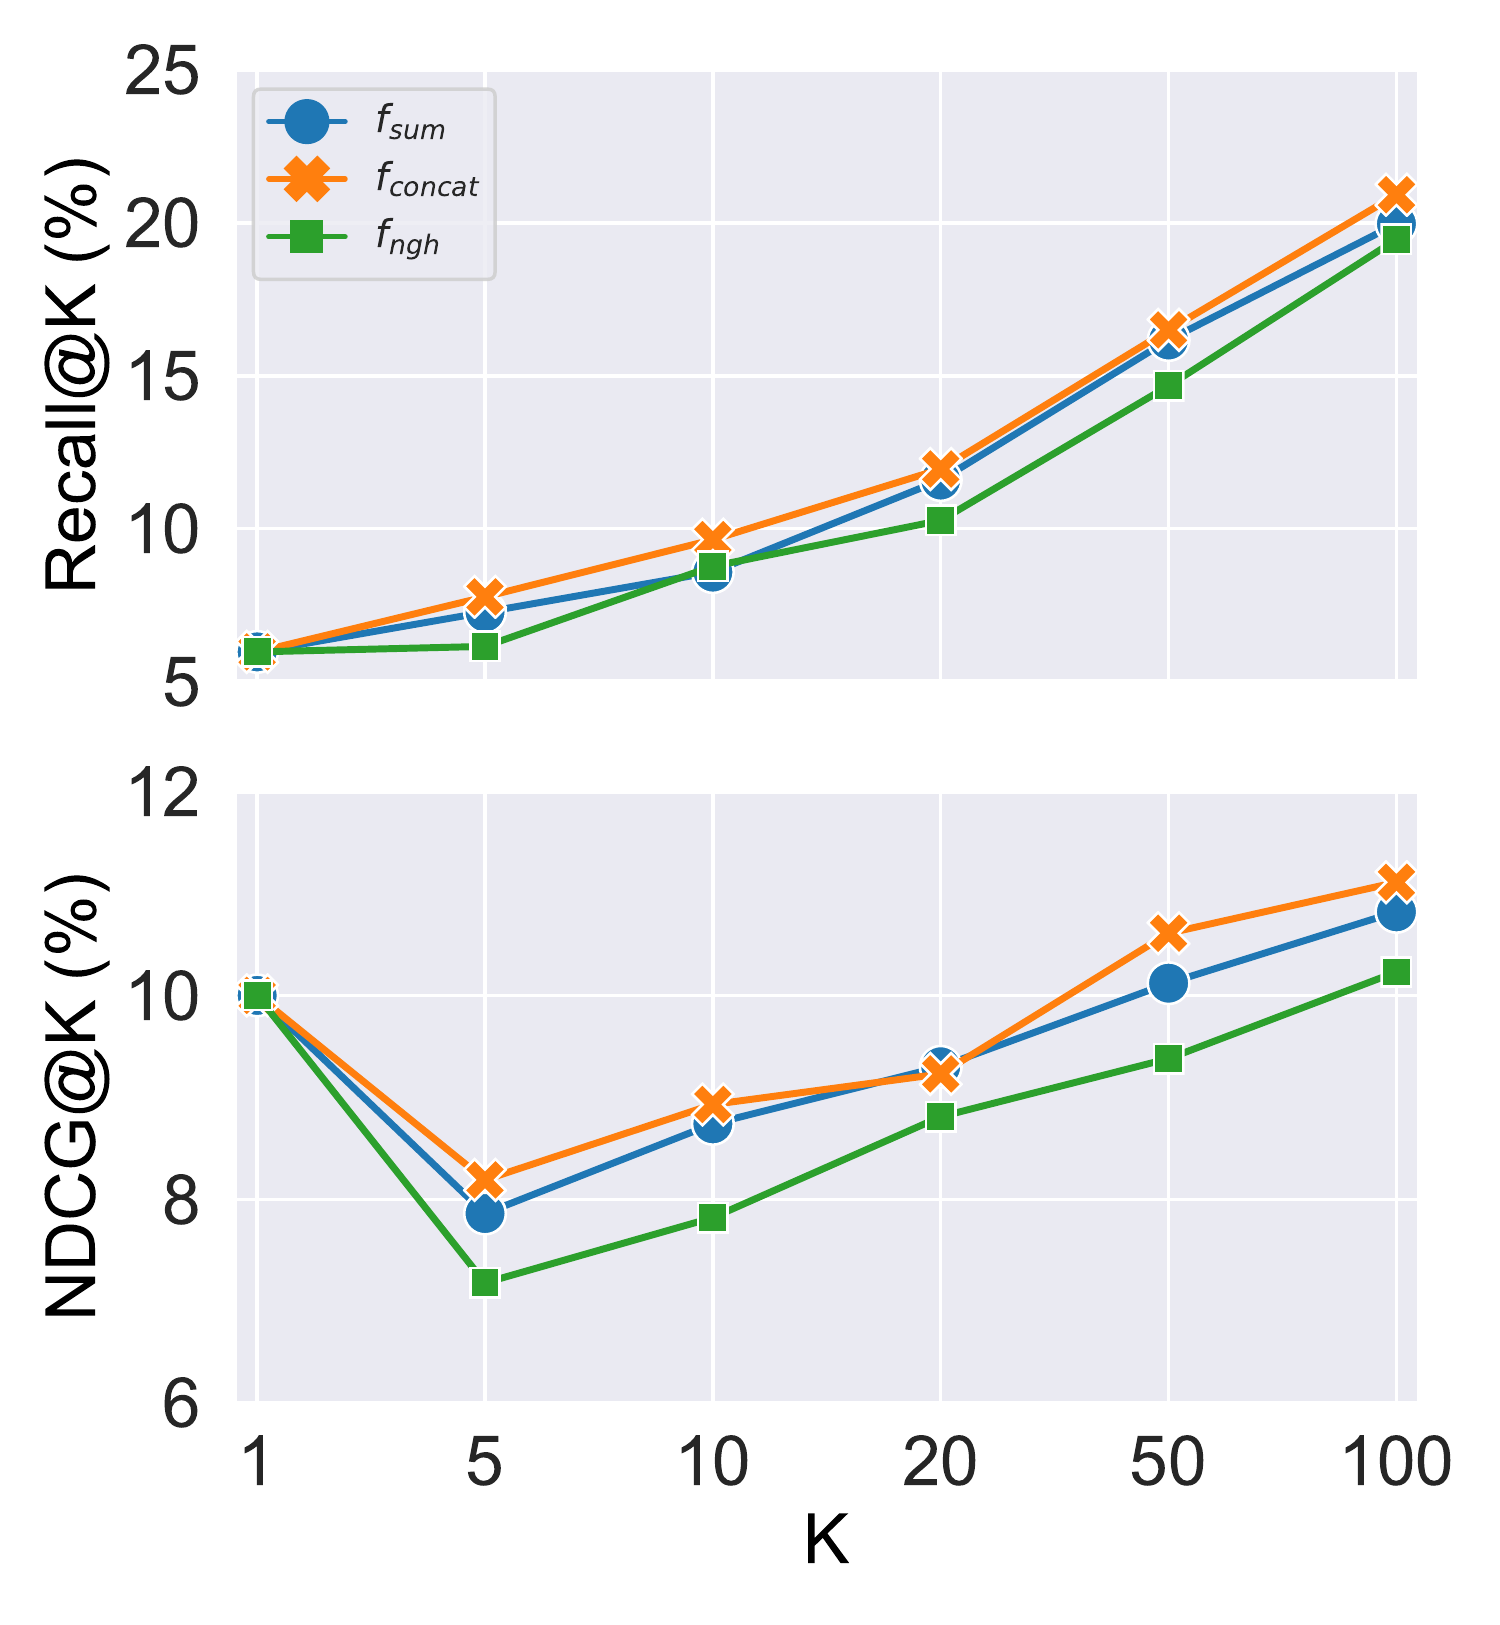}
    \end{minipage}
    }
    \subfigure[ \quad Movie]{
    \begin{minipage}{0.235\textwidth}
      \includegraphics[width=1.75in]{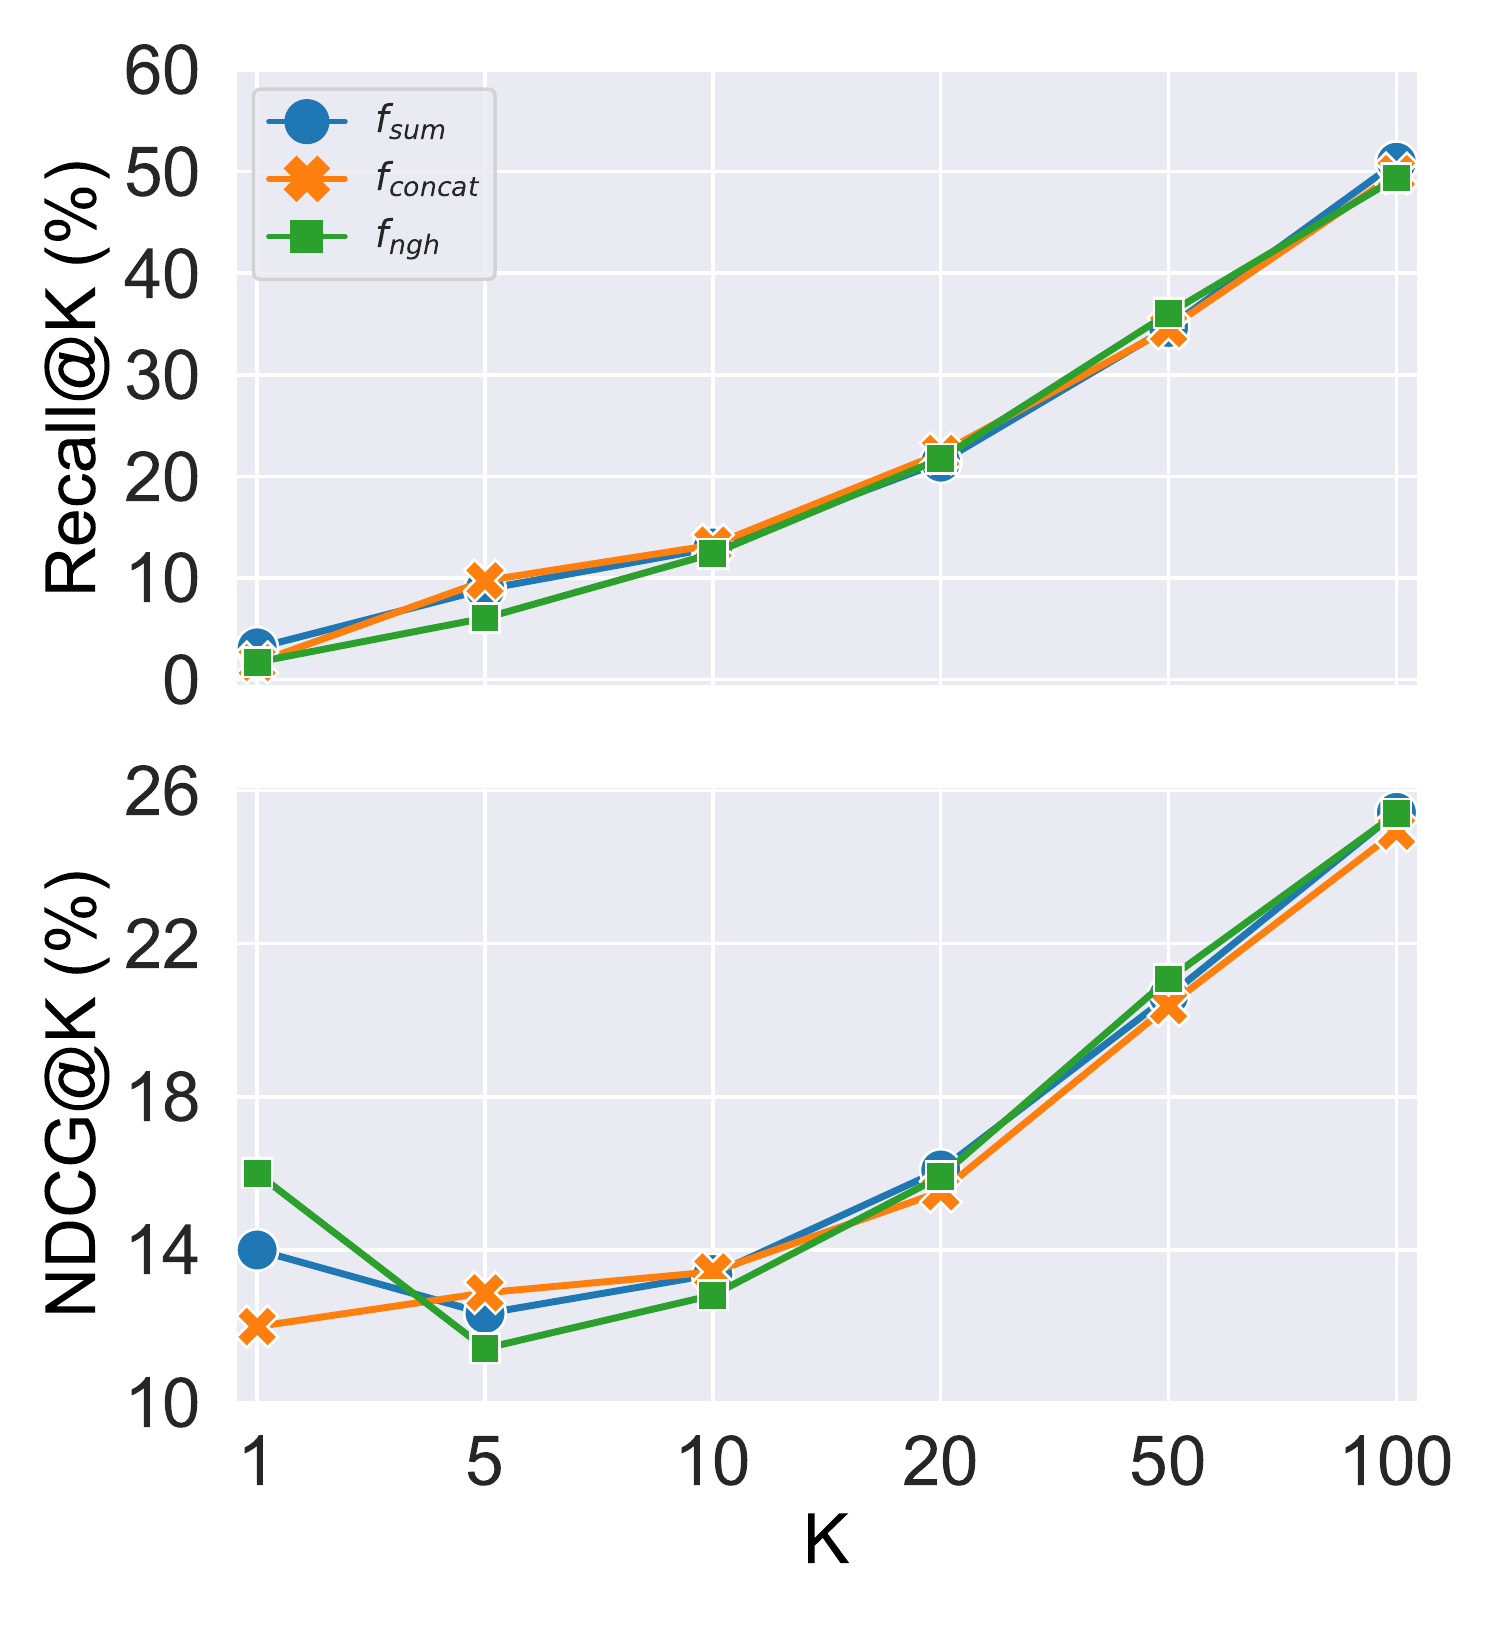}
    \end{minipage}
    }
    \subfigure[ \quad Restaurant]{
    \begin{minipage}{0.235\textwidth}
      \includegraphics[width=1.75in]{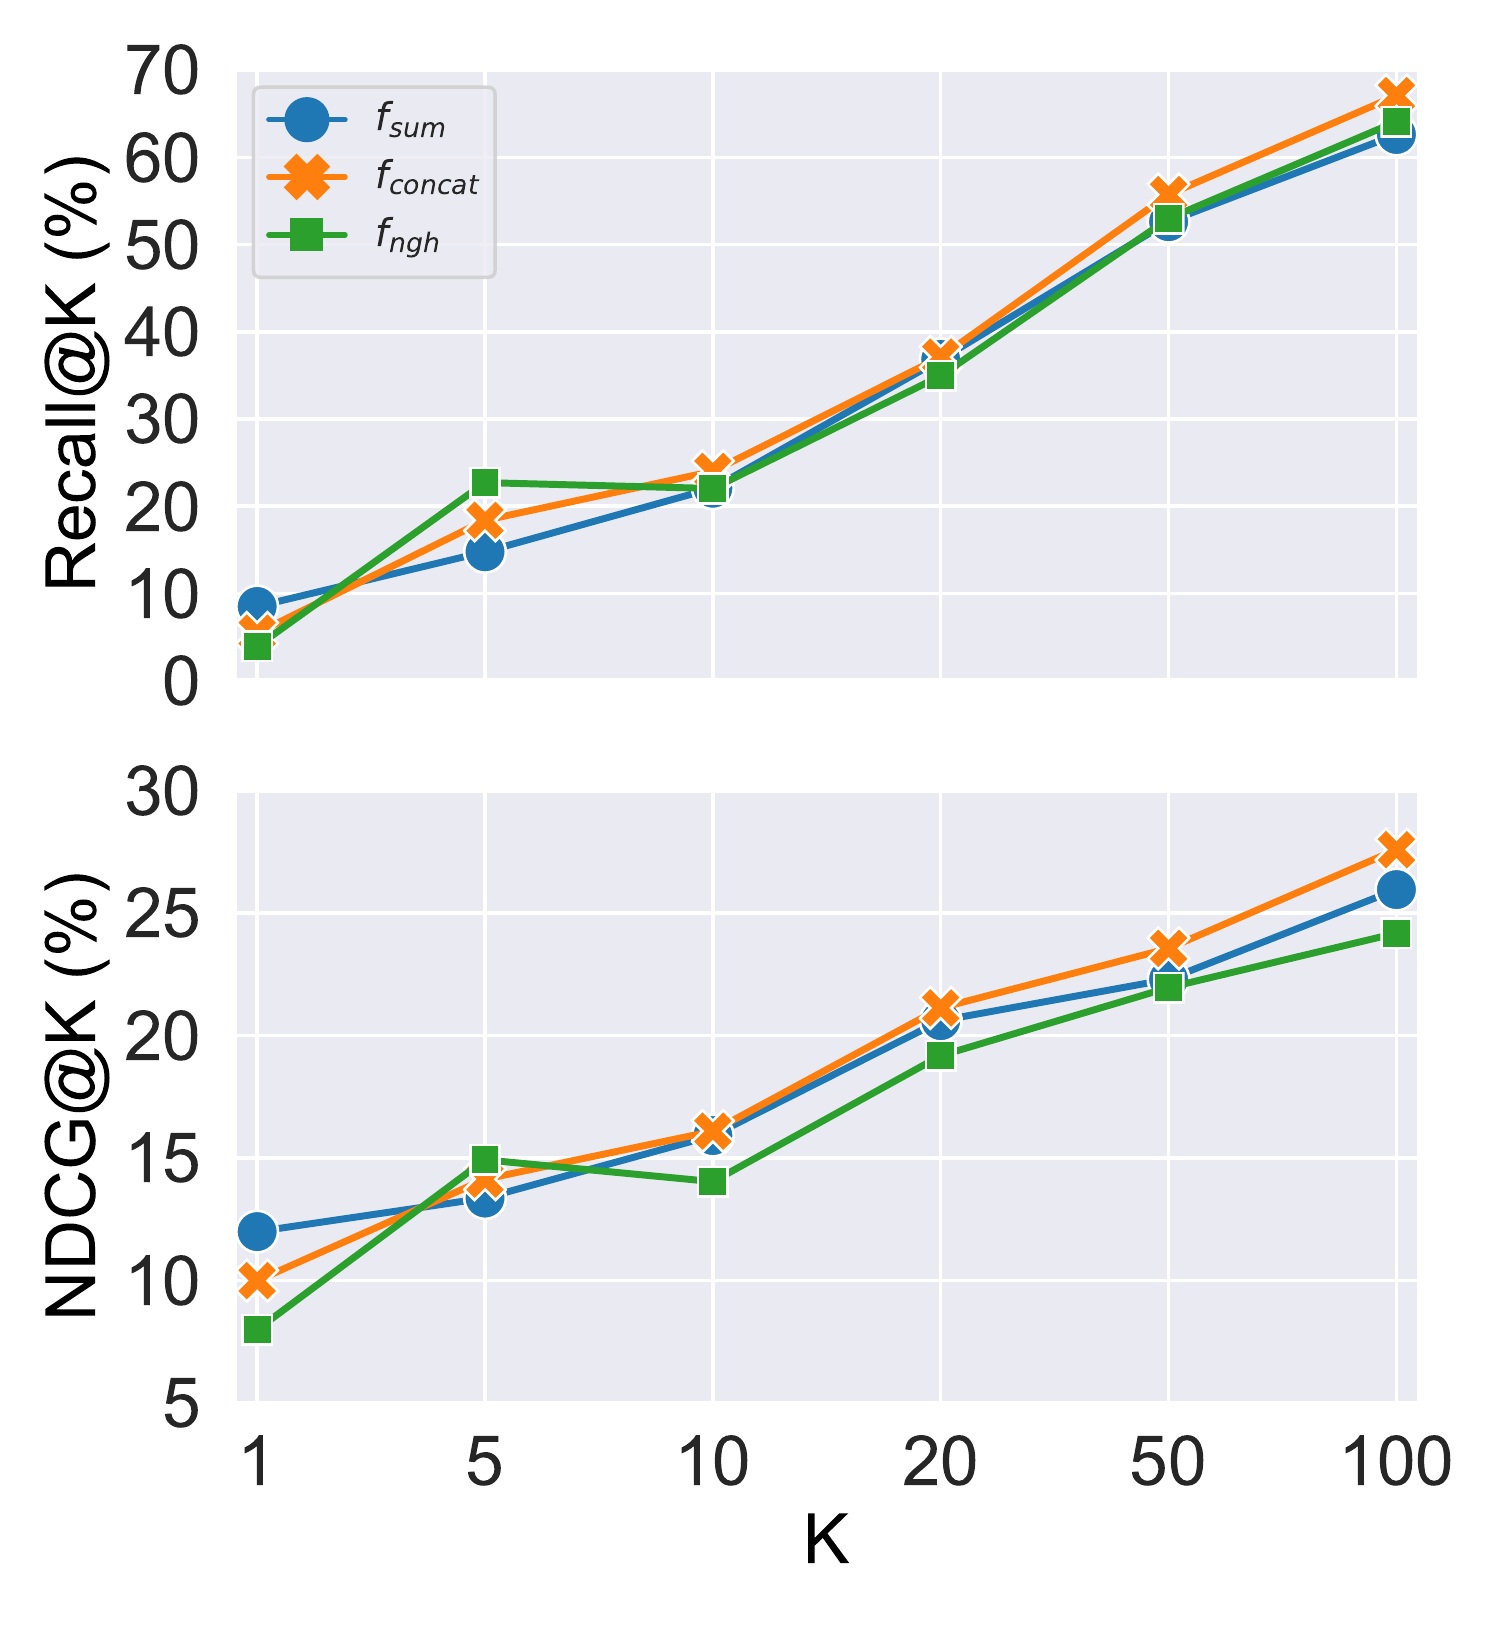}
    \end{minipage}
    }
\caption{Average results of Recall@$K$ and NDCG@$K$ with dfferent aggregators.}
\label{fig:topk_aggregator}
\end{figure*}

\subsubsection{\textbf{CTR Prediction Results of Different Aggregators.}}
We attach the AUC and F1 metrics for CTR prediction with different aggregators in Table~\ref{tb:agg_auc}.

\begin{table}[ht]
\centering
\caption{CTR prediction of different aggregators $g(\cdot)$ (\%).}
\label{tb:agg_auc}
\setlength{\tabcolsep}{5.8mm}{
\begin{tabular}{c|c c c}
\toprule
  Dataset & $g_{sum}$  & $g_{concat}$  & $g_{neighbor}$  \\
\midrule
\midrule
  MS-AUC  &{82.56}     &{\textbf{83.95}}   &{81.01}\\ 
  MS-F1   &{73.27}     &{\textbf{74.82}}   &{72.59}\\ 
\midrule  
  BK-AUC  &{74.18}     &{\textbf{75.75}}   &{74.77}\\ 
  BK-F1   &{66.15}     &{\textbf{67.48}}   &{67.21}\\ 
\midrule
  MV-AUC  &{98.12}     &{\textbf{98.27}}   &{97.73}\\ 
  MV-F1   &{93.87}     &{\textbf{94.14}}   &{93.14}\\ 
\midrule  
  RT-AUC  &{90.54}     &{\textbf{90.68}}   &{90.41}\\ 
  RT-F1   &{83.21}     &{\textbf{83.39}}   &{83.11}\\ 
\bottomrule
\end{tabular}}
\end{table}

\subsection{CG-KGR Model Performance with Knowledge Extraction Hops}

\subsubsection{\textbf{Top-$K$ Recomendation Results of Different Knowledge Extraction Hops.}}
Experimental results of knowledge extraction hop depths on Top-$K$ recomendation are reported in Figure~\ref{fig:topk_layer}.

\begin{figure*}[hb]
\hspace{-0.15in}
  \subfigure[ \quad Music]{  
    \begin{minipage}{0.235\textwidth}
      \includegraphics[width=1.75in]{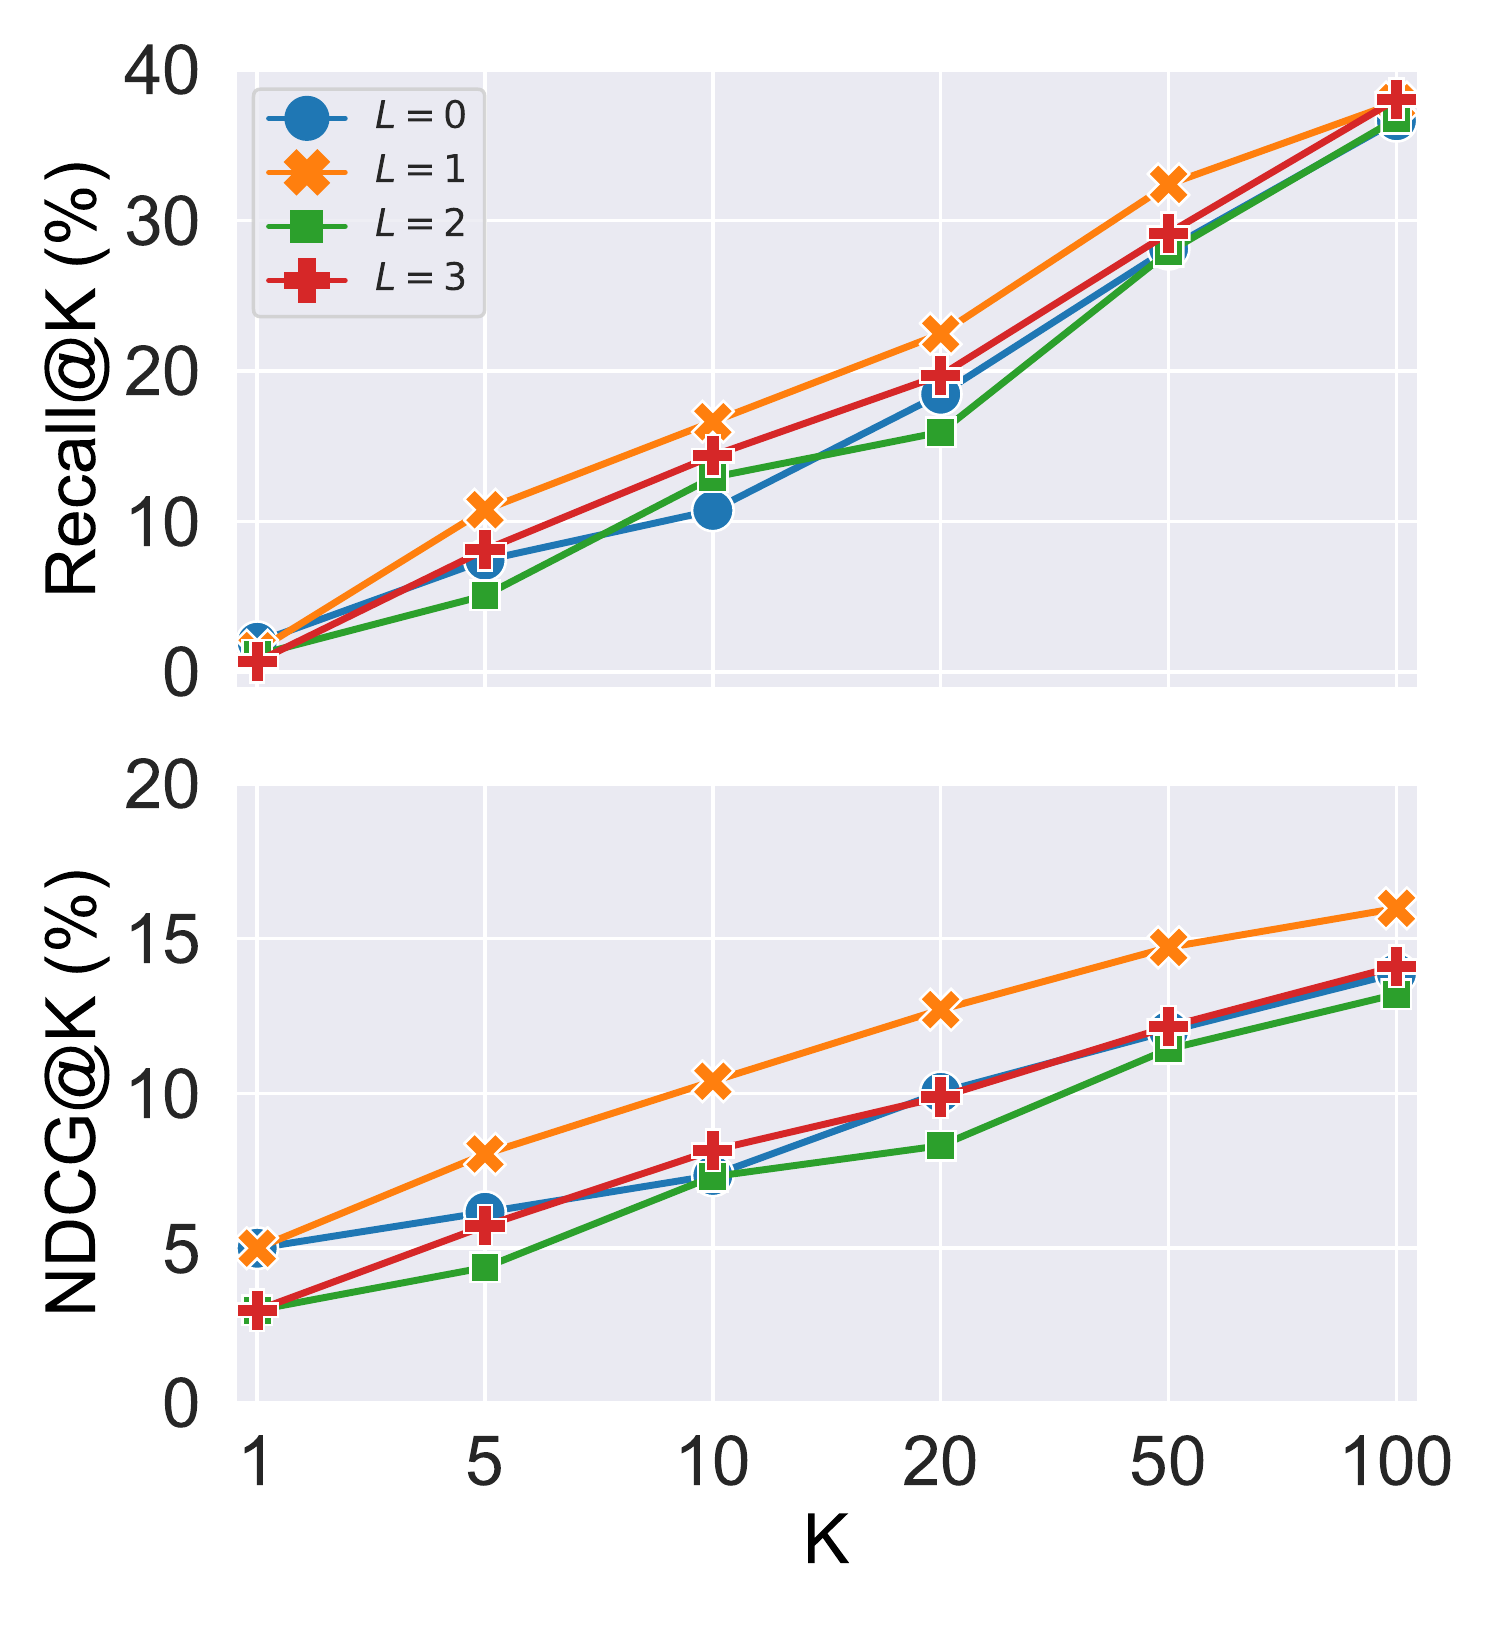}
    \end{minipage}
    }
  \subfigure[ \quad Book]{  
    \begin{minipage}{0.235\textwidth}
      \includegraphics[width=1.75in]{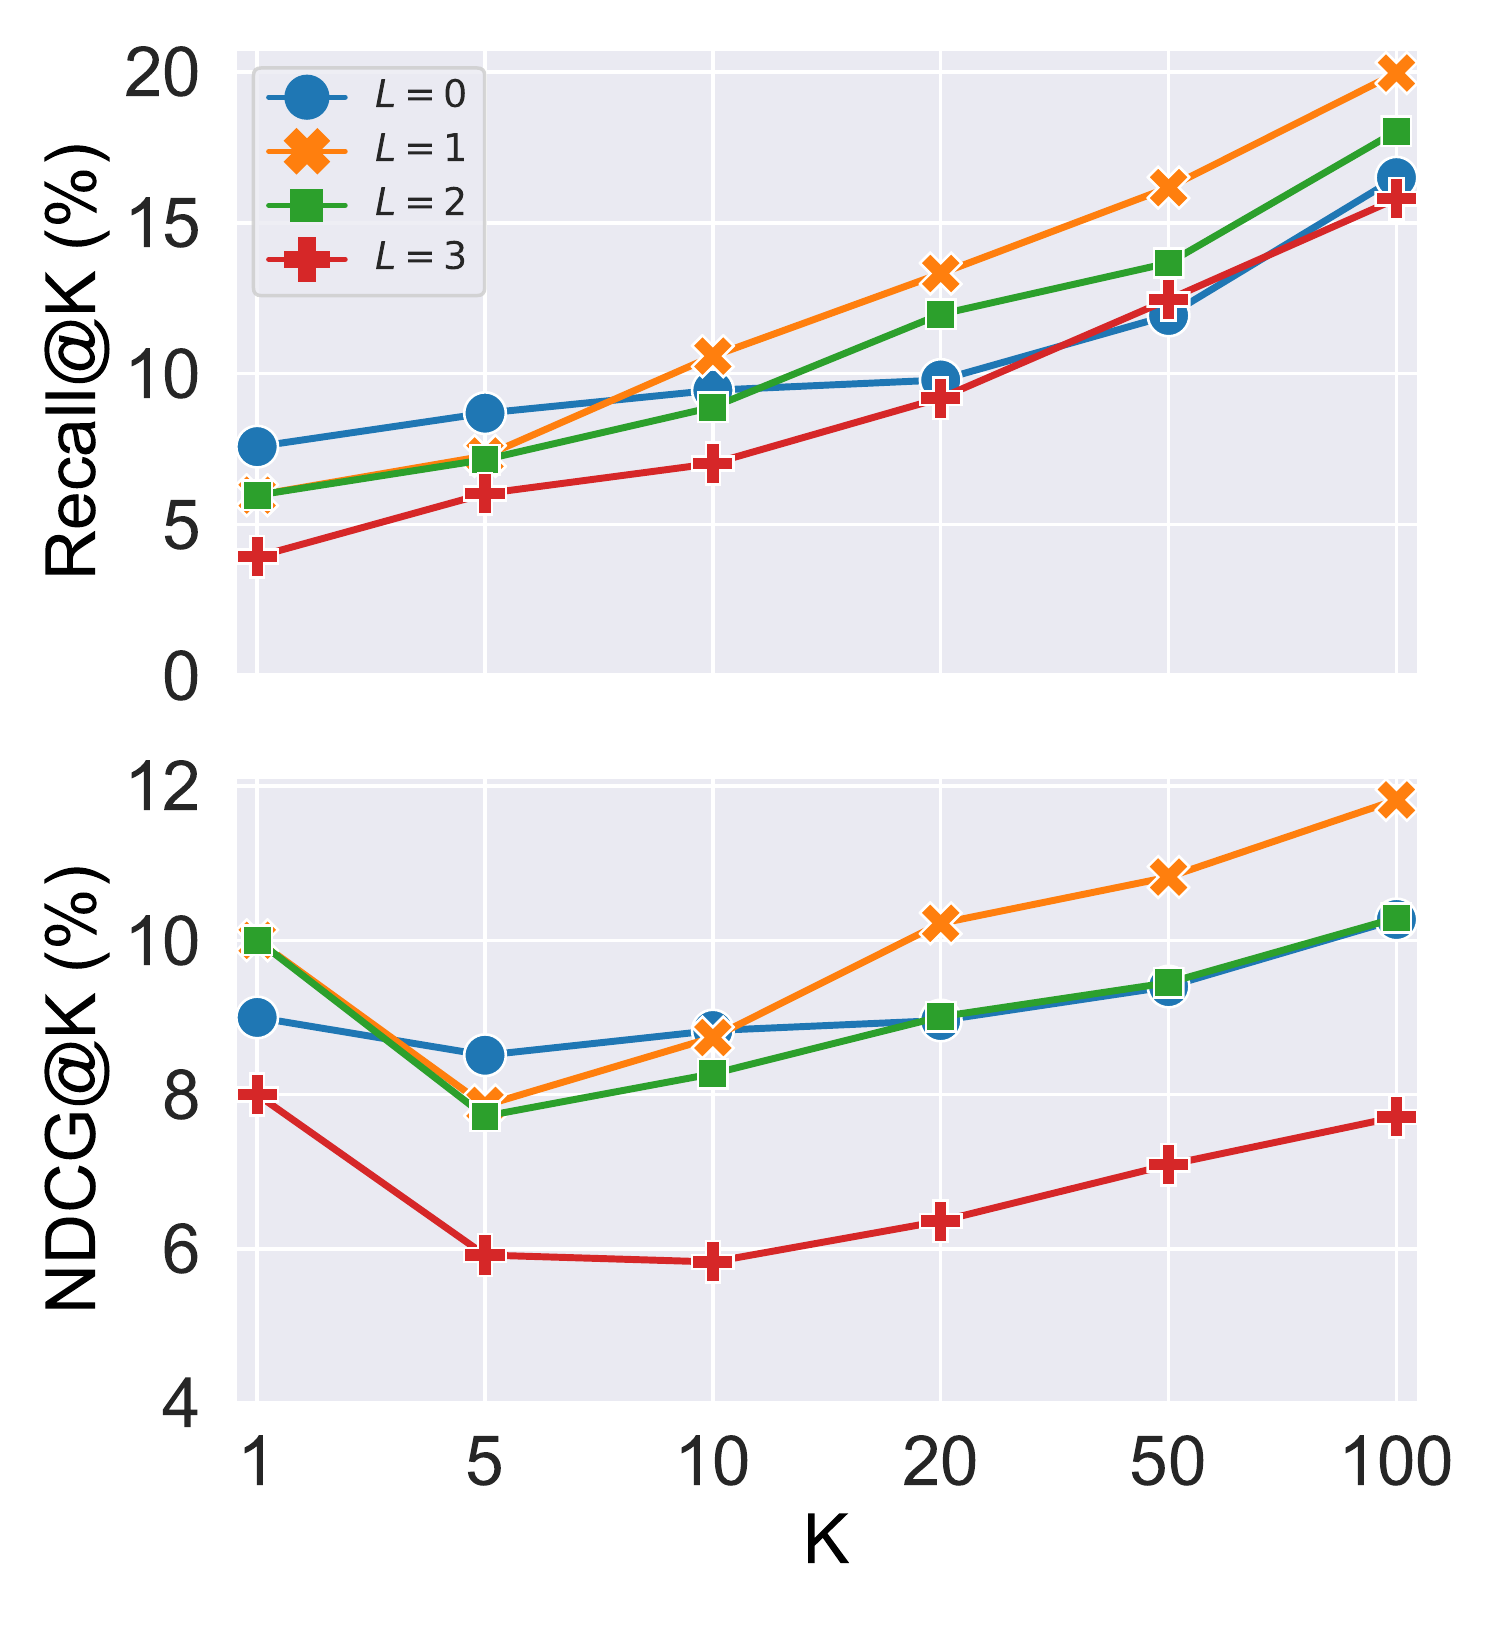}
    \end{minipage}
    }
    \subfigure[ \quad Movie]{
    \begin{minipage}{0.235\textwidth}
      \includegraphics[width=1.75in]{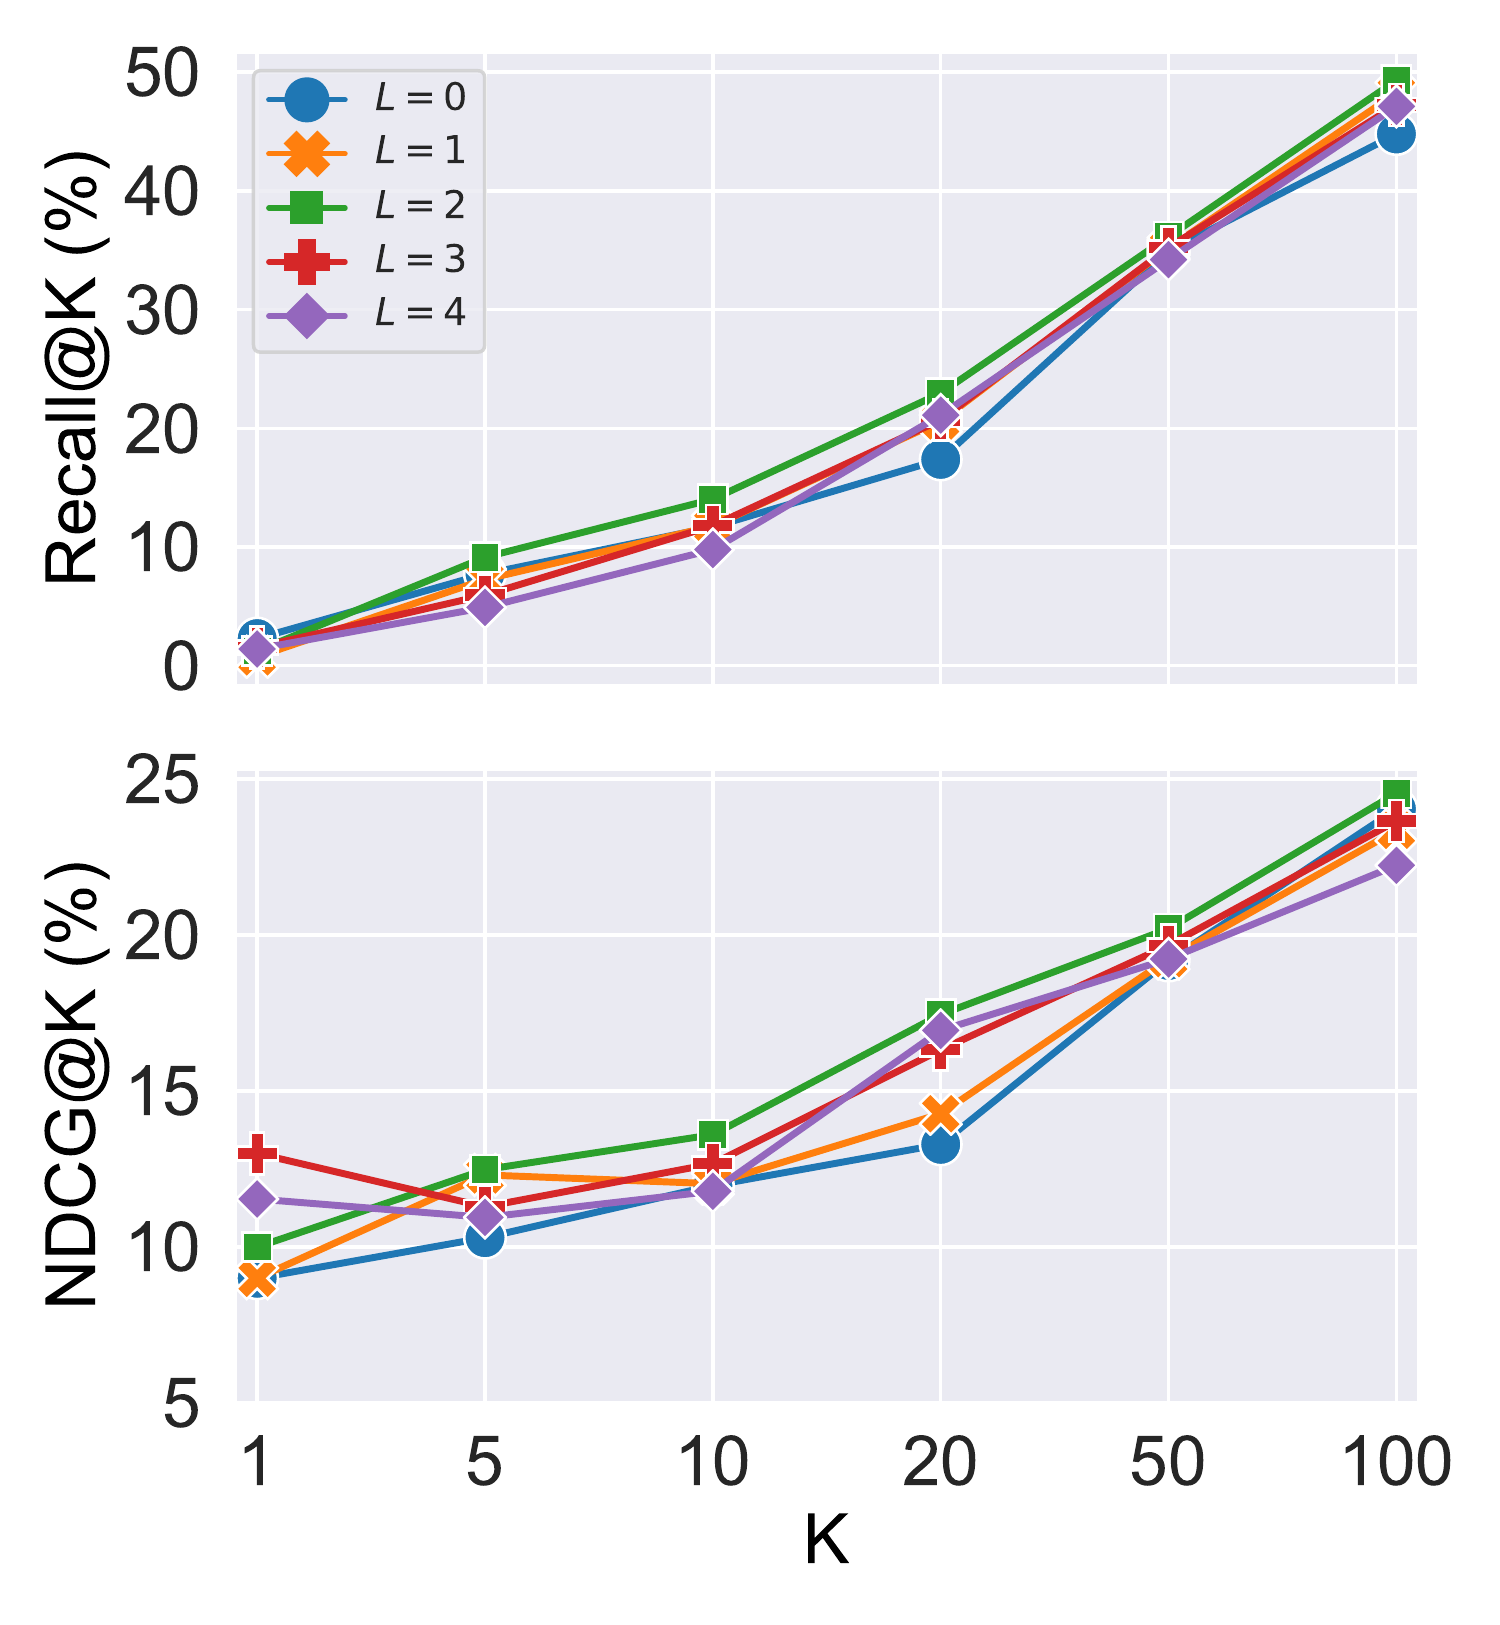}
    \end{minipage}
    }
    \subfigure[ \quad Restaurant]{
    \begin{minipage}{0.235\textwidth}
      \includegraphics[width=1.75in]{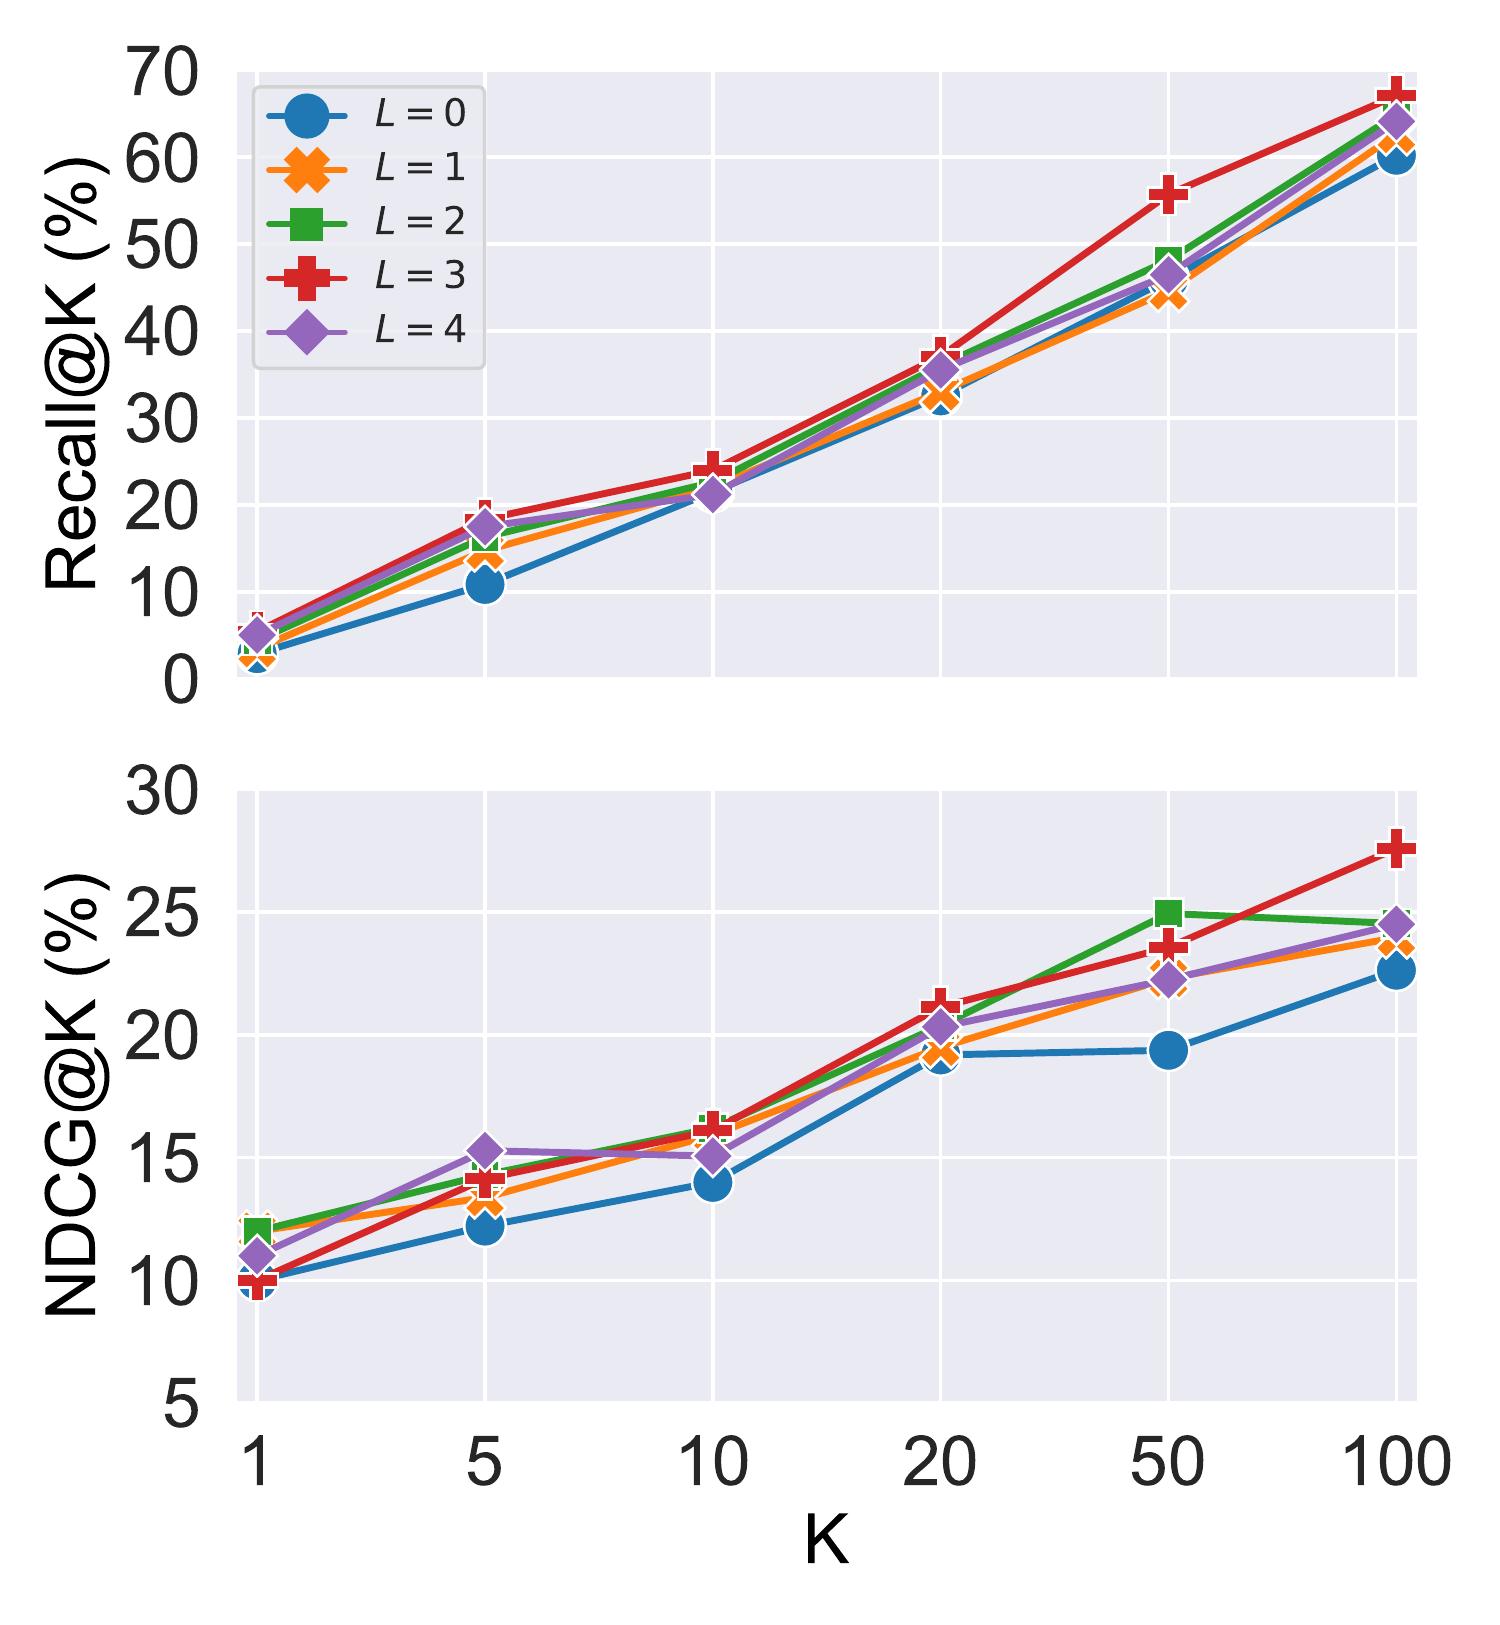}
    \end{minipage}
    }
\caption{Average results of Recall@K and NDCG@K with dfferent hop depths.}
\label{fig:topk_layer}
\end{figure*}

\subsubsection{\textbf{CTR Prediction Results of Different Knowledge Extraction Hops.}}
We attach the CTR Prediction of different extraction hops \textit{w.r.t} AUC and F1 in Table~\ref{tab:layer_auc}.

\begin{table}[H]
\centering
\caption{CTR prediction of different hop depths $L$ (\%).}
\label{tab:layer_auc}
\setlength{\tabcolsep}{3.2mm}{
\begin{tabular}{c | c c c c c}
\toprule
    Dataset & $L = 0$  & $L = 1$  &  $L = 2$  & $L = 3$  & $L = 4$ \\
\midrule
\midrule
  MS-AUC  &{82.47}&{\textbf{83.95}}&{82.48}&{83.13}&{-}\\
  MS-F1   &{72.95}&{\textbf{74.82}}&{72.92}&{73.11}&{-}\\
\midrule  
  BK-AUC  &{74.36}&{\textbf{75.75}}&{75.02}&{74.83}&{-}\\
  BK-F1   &{65.93}&{\textbf{67.25}}&{66.83}&{66.46}&{-}\\
\midrule
  MV-AUC  &{96.74}&{98.19}&{\textbf{98.27}}&{98.18}&{98.20}\\
  MV-F1   &{92.34}&{94.01}&{\textbf{94.14}}&{94.07}&{94.03}\\
\midrule  
  RT-AUC  &{90.27}&{90.42}&{90.59}&{\textbf{90.68}}&{89.98}\\
  RT-F1   &{82.54}&{83.07}&{83.33}&{\textbf{83.39}}&{82.70}\\
\bottomrule
\end{tabular}}
\end{table}

\subsection{Selection of Collaborative Encoders}
\subsubsection{\textbf{Top-K recommendation Results of Different $f(\cdot)$.}}
We also evaluate the selection of different user-item collaborative encoders in the Top-$K$ recommendation tasks and decipt the results in Figure~\ref{fig:ui_rep}.
\begin{figure*}[b]
\hspace{-0.15in}
  \subfigure[ \quad Music]{  
    \begin{minipage}{0.235\textwidth}
      \includegraphics[width=1.75in]{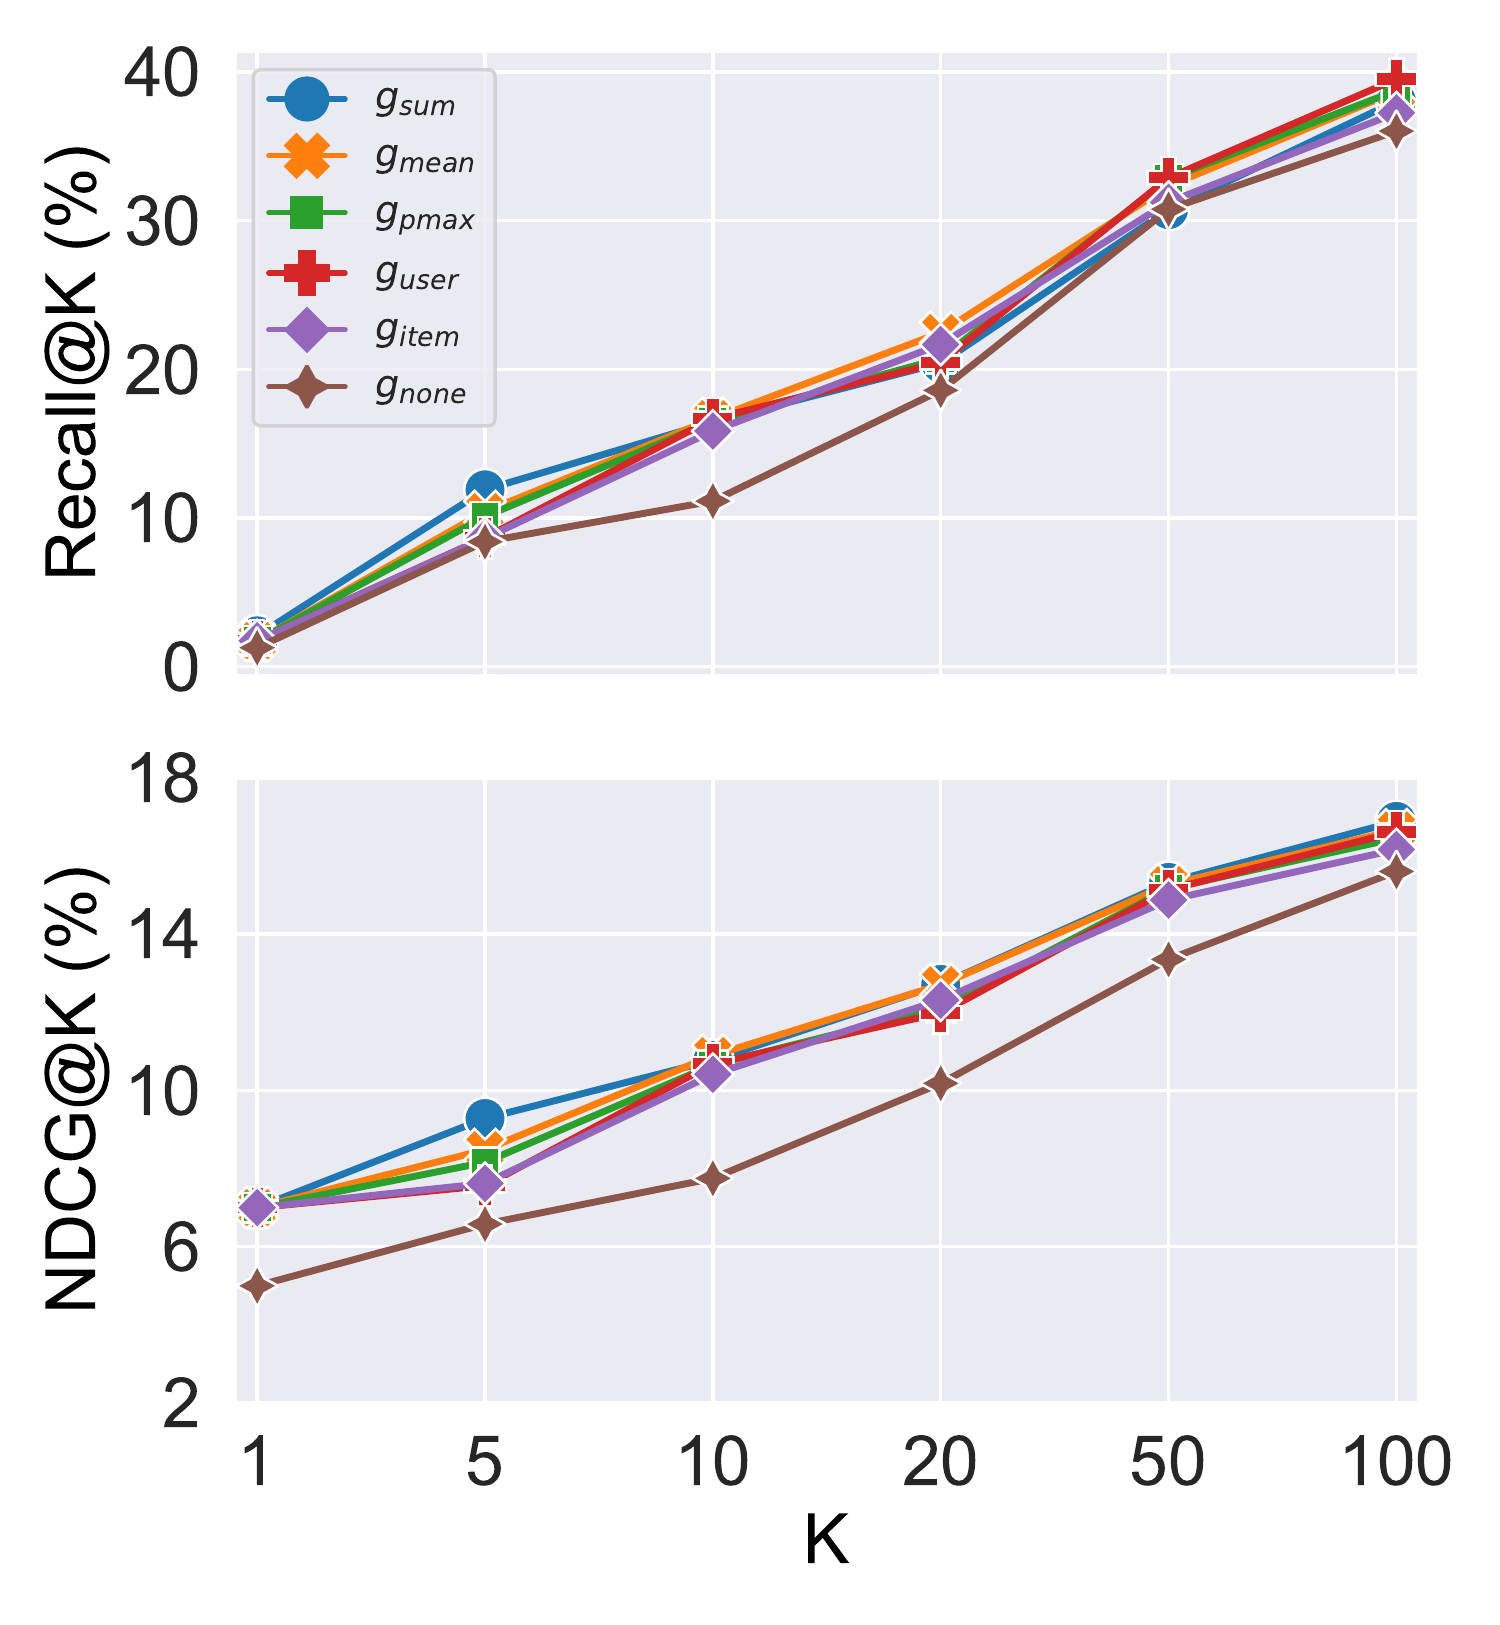}
    \end{minipage}
    }
  \subfigure[ \quad Book]{  
    \begin{minipage}{0.235\textwidth}
      \includegraphics[width=1.75in]{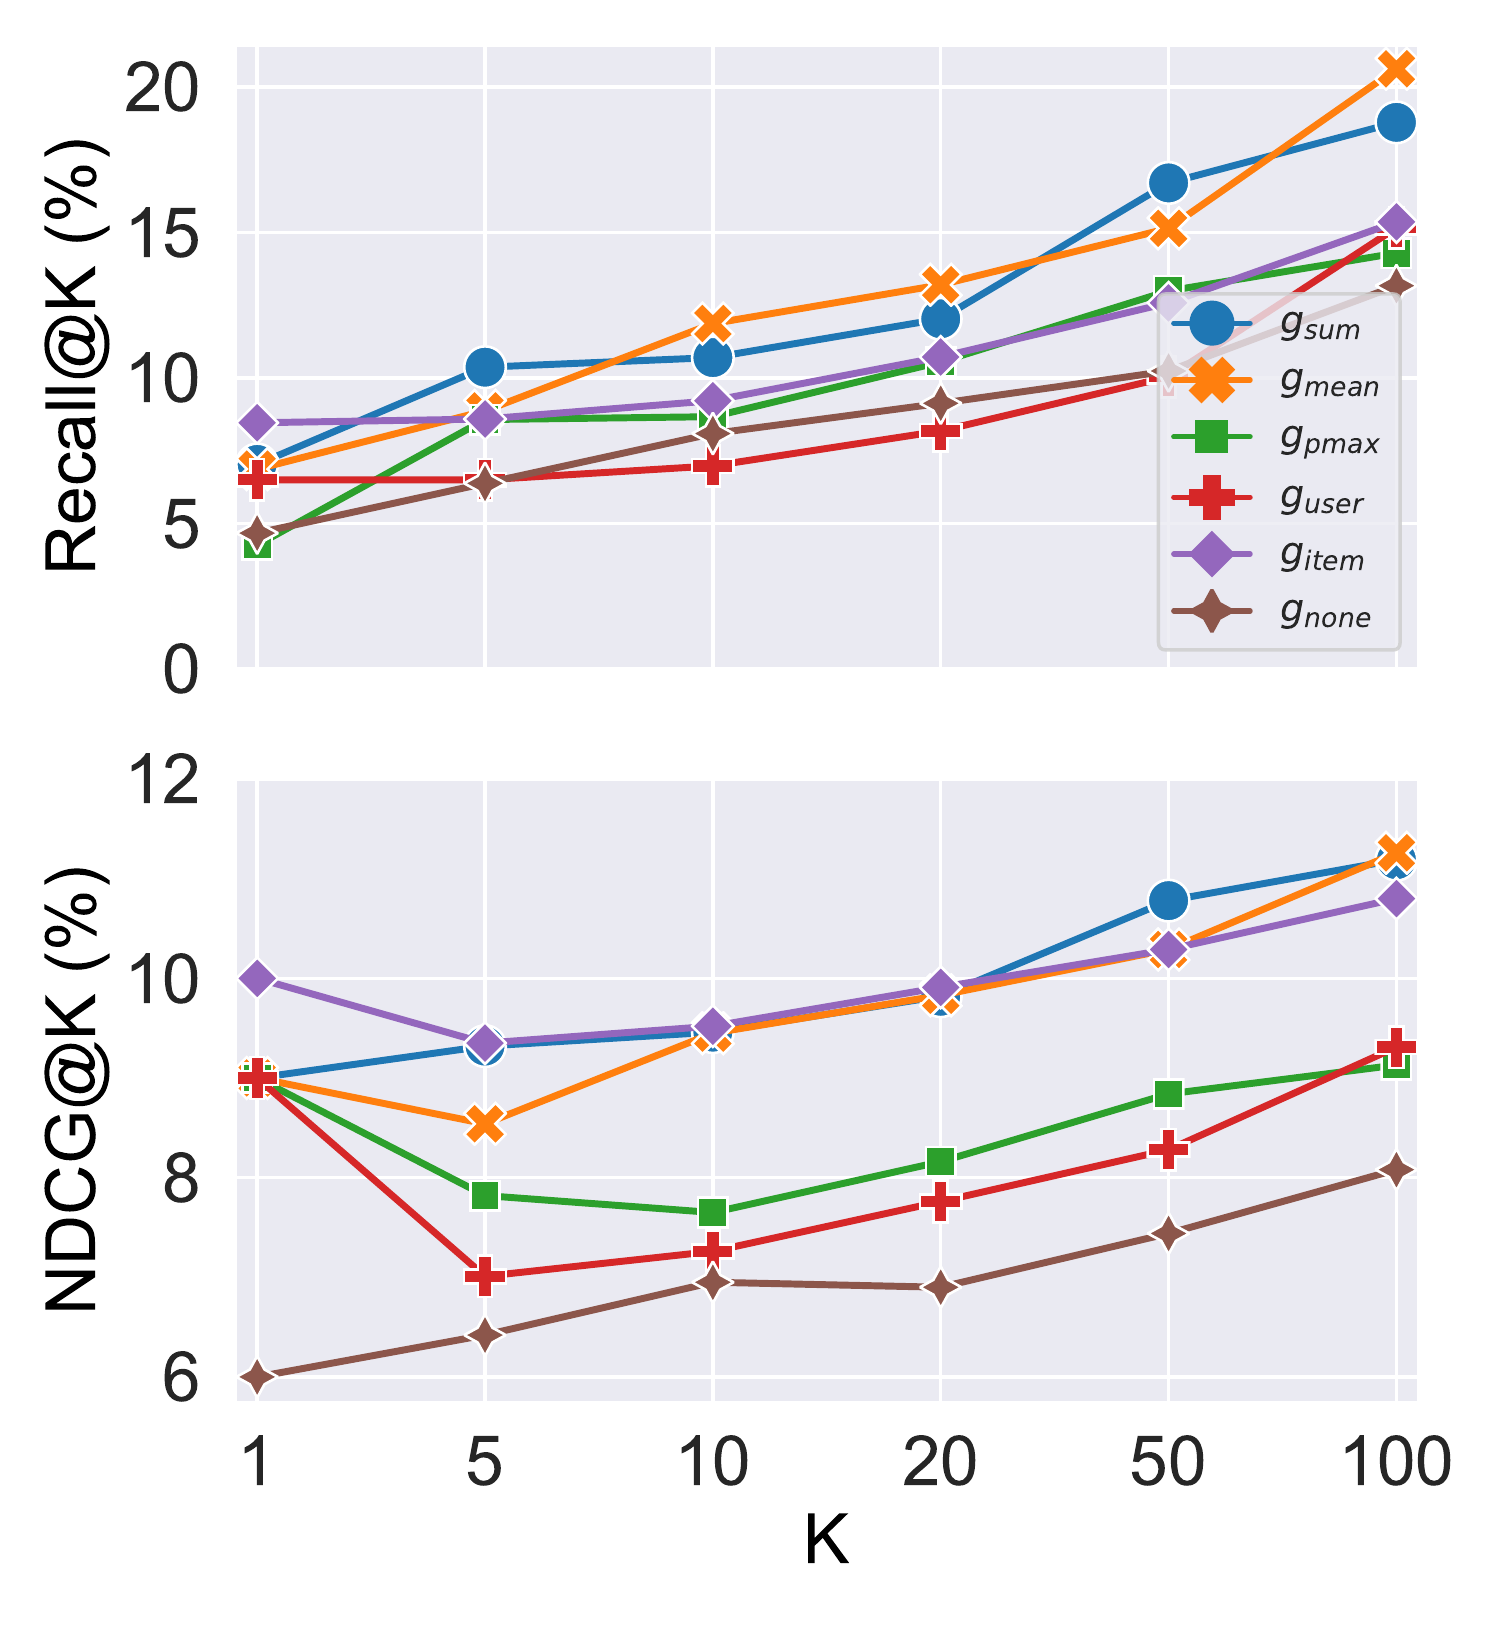}
    \end{minipage}
    }
    \subfigure[ \quad Movie]{
    \begin{minipage}{0.235\textwidth}
      \includegraphics[width=1.75in]{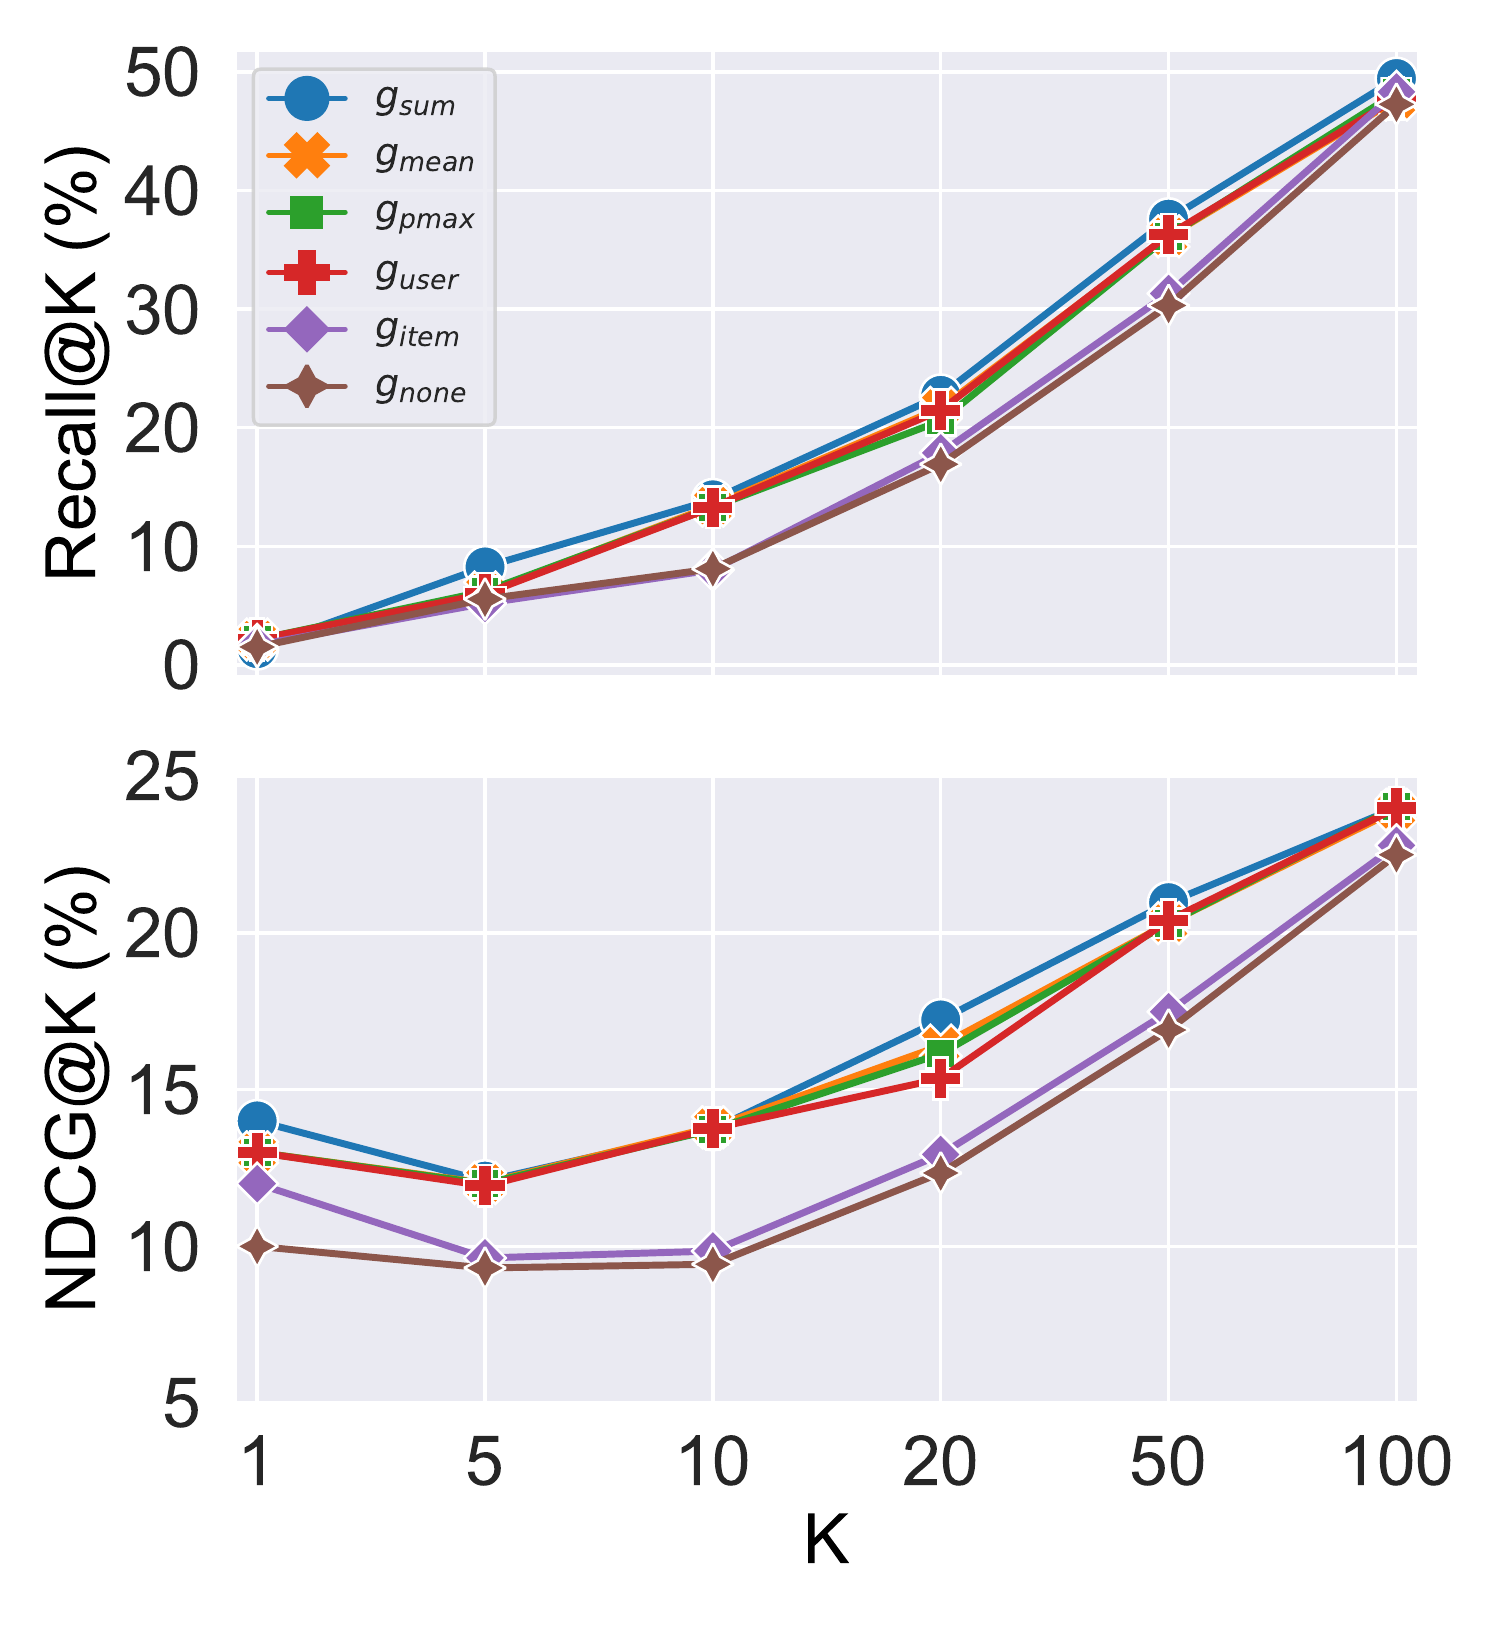}
    \end{minipage}
    }
    \subfigure[ \quad Restaurant]{
    \begin{minipage}{0.235\textwidth}
      \includegraphics[width=1.75in]{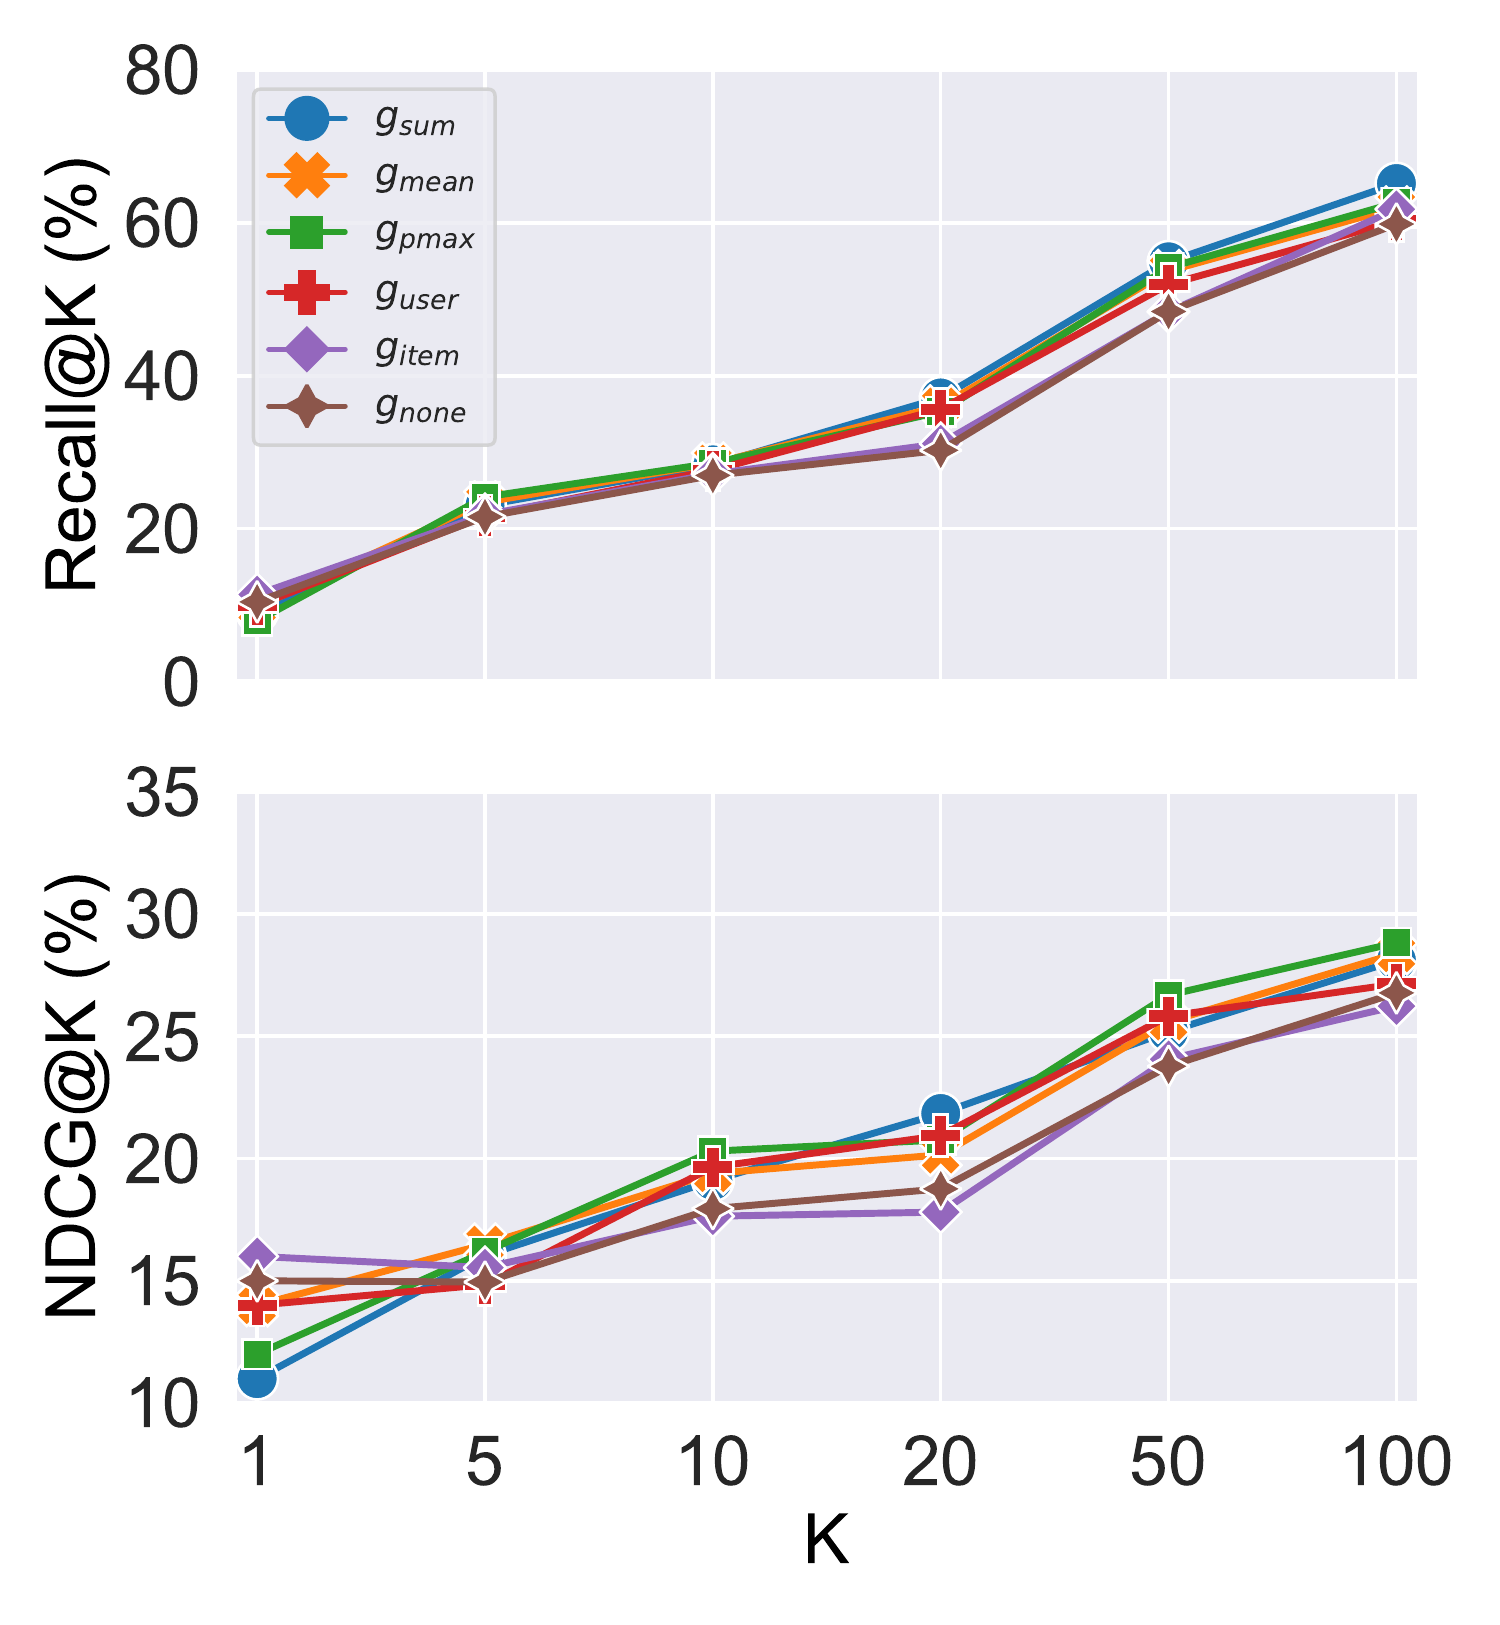}
    \end{minipage}
    }
\caption{Average results of Recall@$K$ and NDCG@$K$ with different collaborative encoder $f$.}
\label{fig:ui_rep}
\end{figure*}

\subsubsection{\textbf{CTR Prediction Results of Different $f(\cdot)$.}}
We attach the AUC and F1 metrics for CTR prediction with different collaborative encoder $f(\cdot)$ in Table~\ref{tb:repr_auc}.

\begin{table}[ht]
\centering
\caption{CTR prediction of different collaborative encoder $f(\cdot)$ (\%).}
\label{tb:repr_auc}
\setlength{\tabcolsep}{5.8mm}{
\begin{tabular}{c|c c c}
\toprule
  Dataset & $f_{sum}$  & $f_{mean}$  & $f_{pmax}$  \\
\midrule
\midrule
  MS-AUC  &{83.56}     &{\textbf{83.95}}   &{82.97}\\ 
  MS-F1   &{74.27}     &{\textbf{74.82}}   &{72.95}\\ 
\midrule  
  BK-AUC  &{75.23}     &{\textbf{75.75}}   &{74.47}\\ 
  BK-F1   &{66.21}     &{\textbf{67.48}}   &{65.86}\\ 
\midrule
  MV-AUC  &{confirmed 98.33}     &{\textbf{98.27}}   &{96.33}\\ 
  MV-F1   &{94.23}     &{\textbf{94.14}}   &{93.24}\\ 
\midrule  
  RT-AUC  &{89.46}     &{\textbf{90.68}}   &{88.16}\\ 
  RT-F1   &{82.29}     &{\textbf{83.39}}   &{82.21}\\ 
\bottomrule
\end{tabular}}
\end{table}

\subsection{Details of Ablation Study of CG-KGR Model on CTR Prediction and Top-K Recommendation}
\label{app:Ablation_Study_CGKGR}

\begin{table}[ht]
\centering
\caption{Ablation study on CTR prediction (\%).}
\label{tab:ab_ctr}
\setlength{\tabcolsep}{0.5mm}{
\begin{tabular}{c| c | c | c | c  | c |c}
\toprule
 Dataset      &   w/o UI &  w/o KG  &  w/o ATT  & w/o CG & w/o HE & Best \\
\midrule
\midrule
         {\scriptsize MS-AUC}  & {\scriptsize 75.50}{\,{\tiny(-10.05\%)}}      
                            & {\scriptsize 79.47}{\,{\tiny(-5.33\%)}}      
                            & {\scriptsize 79.81}{\,{\tiny(-4.92\%)}}  
                            & {\scriptsize 81.71}{\,{\tiny(-2.67\%)}}  
                            & {\scriptsize 83.95}{\,{\tiny(-)}} 
                            & {\textbf{83.95}} \\
        {\scriptsize MS-F1} & {\scriptsize 68.76}{\,{\tiny(-10.78\%)}}    
                            & {\scriptsize 70.36}{\,{\tiny(-6.01\%)}}      
                            & {\scriptsize 71.97}{\,{\tiny(-3.82\%)}}   
                            & {\scriptsize 72.85}{\,{\tiny(-2.63\%)}}  
                            & {\scriptsize 74.82}{\,{\tiny(-)}}  
                            & {\textbf{74.82}} \\   
 \midrule 
        {\scriptsize BK-AUC}& {\scriptsize 68.29}{\,{\tiny(-10.36\%)}}    
                            & {\scriptsize 74.76}{\,{\tiny(-1.86\%)}}   
                            & {\scriptsize 74.44}{\,{\tiny(-2.28\%)}}  
                            & {\scriptsize 74.69}{\,{\tiny(-1.40\%)}}  
                            & {\scriptsize 75.75}{\,{\tiny(-)}}
                            & {\textbf{75.75}} \\
        {\scriptsize BK-F1} & {\scriptsize 63.71}{\ \,{\tiny(-5.26\%)}}   
                            & {\scriptsize 65.60}{\,{\tiny(-2.45\%)}} 
                            & {\scriptsize 66.08}{\,{\tiny(-1.74\%)}}   
                            & {\scriptsize 66.55}{\,{\tiny(-1.38\%)}} 
                            & {\scriptsize 67.48}{\,{\tiny(-)}}
                            & {\textbf{67.48}} \\   
 \midrule
        {\scriptsize MV-AUC}& {\scriptsize 97.90}{\,{\tiny(-0.39\%)}}       
                            & {\scriptsize 98.21}{\,{\tiny(-0.07\%)}}      
                            & {\scriptsize 98.22}{\,{\tiny(-0.06\%)}}     
                            & {\scriptsize 98.26}{\,{\tiny(-0.01\%)}}   
                            & {\scriptsize 98.19}{\,{\tiny(-0.01\%)}}
                            &{\textbf{98.27}} \\
        {\scriptsize MV-F1} & {\scriptsize 93.53}{\,{\tiny(-0.63\%)}}       
                            & {\scriptsize 94.01}{\,{\tiny(-0.01\%)}}       
                            & {\scriptsize 93.94}{\,{\tiny(-0.02\%)}}  
                            & {\scriptsize 94.12}{\,{\tiny(-0.02\%)}}  
                            & {\scriptsize 94.01}{\,{\tiny(-0.01\%)}} 
                            &{\textbf{94.14}} \\   
 \midrule
        {\scriptsize RT-AUC}& {\scriptsize 85.71}{\,{\tiny(-5.49\%)}}     
                            & {\scriptsize 90.53}{\,{\tiny(-1.10\%)}}    
                            & {\scriptsize 90.53}{\,{\tiny(-1.10\%)}}   
                            & {\scriptsize 90.61}{\,{\tiny(-0.08\%)}}     
                            & {\scriptsize 90.42}{\,{\tiny(-0.03\%)}}
                            &{\textbf{90.68}} \\
        {\scriptsize RT-F1} & {\scriptsize 79.41}{\,{\tiny(-4.68\%)}}   
                            & {\scriptsize 83.02}{\,{\tiny(-0.35\%)}}     
                            & {\scriptsize 83.12}{\,{\tiny(-0.23\%)}}    
                            & {\scriptsize 83.32}{\,{\tiny(-0.08\%)}}
                            & {\scriptsize 83.07}{\,{\tiny(-0.04\%)}} 
                            &{\textbf{83.39}} \\    
\bottomrule
\end{tabular}}
\end{table}

We conduct the ablation study of CG-KGR model on both CTR prediction and Top-K recommendation. We report the AUC and F1 in Table~\ref{tab:ab_ctr}.
